# Supplementary material for: Convert widespread paraelectric perovskite to ferroelectrics
Source: arXiv:2204.00758 source file (2022-04-02)
Supplement: Supplementary file 1 [file supplementary_materials_final.pdf]

# Supplemental Materials for "Convert widespread paraelectric perovskite to ferroelectrics"

Hongwei Wang,[1,2] Fujie Tang,[1] Massimiliano Stengel,[3,4] Hongjun Xiang,[5] Qi An,[6] Tony Low,[2] and Xifan Wu[1,7]

[1]*Department of Physics, Temple University, Philadelphia, PA 19122, USA*

[2]*Department of Electrical and Computer Engineering, University of Minnesota, Minneapolis, Minnesota 55455, USA*

[3]*Institut de Ciència de Materials de Barcelona (ICMAB-CSIC), Campus UAB, 08193 Bellaterra, Spain*

[4]*ICREA-Institució Catalana de Recerca i Estudis Avançats, 08010 Barcelona, Spain, USA*

[5]*Key Laboratory of Computational Physical Sciences (Ministry of Education), State Key Laboratory of Surface Physics and Department of Physics, Fudan University, Shanghai 200438, People's Republic of China*

[6]*Department of Chemical and Materials Engineering, University of Nevada-Reno, Reno, Nevada 89557, USA*

[7]*Institute for Computational Molecular Science, Temple University, Philadelphia, PA 19122, USA*

(Dated: March 12, 2022)

## I. COMPUTIONAL METHOD

Ground state total energy minimizations were performed based on density functional theory (DFT) [S1] as implemented in the VASP code package [S2, S3]. The electron exchange correlation was approximated by the Perdew Burke Ernzerhof revised functional for solid (PBEsol) [S4] within the generalized gradient approximation. The electron ion interaction was treated by the projector-augmented wave method [S5] and the plane wave cutoff energy was set to 500 eV [S6] and 700 eV [S7] for oxide and fluoride perovskites respectively. The integration over the Brillouin-zone was discretized on a 6×6×4 Monkhorst k-point mesh for perovskites of both CTO-type and BFO-type space group symmetries. The total energy in DFT minimization and the forces on atoms are considered to be converged when the difference between successive iterations is less than the tolerances of $10^{-7}$ eV and $10^{-3}$ eV/Å respectively. The eigen-frequencies and eigen-modes of phonons are computed via finite difference method facilitated by the PHONOPY software package [S8]. The electronic part of ferroelectric polarization was computed by Berry phase approach based on modern theory of polarization [S9]. For the first-principles calculations under applied electric displacement field ($\boldsymbol{D}$), we have used the open-source ABINIT code package [S10]. In the first-principles with applied $\boldsymbol{D}$ fields, we utilized the norm conserving pseudopotential [S11] and PBEsol exchange correlation functional [S4]. Plane wave expansion cutoff of 800 eV and 4×4×4 Monkhorst k-point mesh were used for numerical integration over the Brillouin-zone. The search for global minimum among various metastable structures were performed by the genetic algorithm as implemented in the Property Analysis and Simulation Package (PASP) for materials [S12].

## II. EFFECTIVE HAMILTONIAN MODEL

The Landau theory is a foundation to describe structure transitions in crystalline solids on the basis of group theory. In this theory, the free energy of the crystal is expanded in powers of order parameters associated with the irreducible representations of the space group of high-symmetry phase. The values of the order parameter at the free-energy minimum determine the allowed space groups of the low-symmetry phase. To describe the structural transition, the unstable phonon modes of high-symmetry phase can be considered as the order parameters to explore structural behaviors for the low-symmetry phase. Therefore, the structural transition between CTO-type and BFO-type perovskites are describable with major unstable phonon modes of their cubic parent structures. The detailed energy terms defined in the main text based on Landau-type expansion for CTO-type and BFO-type structures of $CdHfO_3$ are given by following equation arrays.

In the main text, we show that the energy for CTO-type structure could be written as:

$$
\begin{aligned}
E_{\text{“CTO”}}(\{\eta_i\}) &= \underbrace{a_1(\{\eta_i\})R^{\mathrm{I}^2} + b_1(\{\eta_i\})R^{\mathrm{I}^4} + a_2(\{\eta_i\})\mathcal{T}^2 + b_2(\{\eta_i\})\mathcal{T}^4 + c_1(\{\eta_i\})R^{\mathrm{I}^2}\mathcal{T}^2}_{E^{\mathrm{Rot}}_{\text{“CTO”}}} + \underbrace{\frac{1}{2}(2B_{11}\bar{\eta}^2 + B_{33}\eta_z^2) + 2B_{13}\bar{\eta}\eta_z + B_{12}\bar{\eta}^2}_{E^{\mathrm{Elas}}_{\text{“CTO”}}} \\
&\quad \underbrace{\begin{aligned}&+ a_3(\{\eta_i\})\mathrm{AFE_{xy}}^2 + b_3(\{\eta_i\})\mathrm{AFE_{xy}}^4 + c_2(\{\eta_i\})R^{\mathrm{I}^2}\mathrm{AFE_{xy}}^2 + c_3(\{\eta_i\})\mathcal{T}^2\mathrm{AFE_{xy}}^2 + d_1(\{\eta_i\})R^{\mathrm{I}}\mathcal{T}\mathrm{AFE_{xy}} \\ &+ a_4(\{\eta_i\})\mathrm{FE_z}^2 + b_4(\{\eta_i\})\mathrm{FE_z}^4 + c_4(\{\eta_i\})R^{\mathrm{I}^2}\mathrm{FE_z}^2 + c_5(\{\eta_i\})\mathcal{T}^2\mathrm{FE_z}^2 + c_6(\{\eta_i\})\mathrm{FE_z}^2\mathrm{AFE_{xy}}^2\end{aligned}}_{E^{\mathrm{(A)FE}}_{\text{“CTO”}}} \\
&= E^{\mathrm{Rot}}_{\text{“CTO”}} + E^{\mathrm{Elas}}_{\text{“CTO”}} + E^{\mathrm{(A)FE}}_{\text{“CTO”}} \qquad \text{(S1)}
\end{aligned}
$$

Here we decompose the energy terms for CTO-type structure as follows:

1. The coefficients of these terms in $E^{\mathrm{Rot}}_{\text{“CTO”}}$ could be written as:
   - $a_1(\{\eta_i\}) = l_1 + 2e_1\bar{\eta} + e_2\eta_z$, $a_2(\{\eta_i\}) = l_2 + 2e_3\bar{\eta} + e_4\eta_z$;
   - $b_1(\{\eta_i\}) = m_1 + 2f_1\bar{\eta} + f_2\eta_z$, $b_2(\{\eta_i\}) = m_2 + 2f_3\bar{\eta} + f_4\eta_z$;
   - $c_1(\{\eta_i\}) = n_1 + 2g_1\bar{\eta} + g_2\eta_z$.
2. The coefficients of these terms in $E^{\mathrm{(A)FE}}_{\text{“CTO”}}$ could be written as:
   - $a_3(\{\eta_i\}) = l_3 + 2e_5\bar{\eta} + e_6\eta_z$, $b_3(\{\eta_i\}) = m_3 + 2f_5\bar{\eta} + f_6\eta_z$;
   - $c_2(\{\eta_i\}) = n_2 + 2g_3\bar{\eta} + g_4\eta_z$, $c_3(\{\eta_i\}) = n_3 + 2g_5\bar{\eta} + g_6\eta_z$;
   - $d_1(\{\eta_i\}) = o_1 + 2h_1\bar{\eta} + h_2\eta_z$.
3. The coefficients of the additional terms in $E^{\mathrm{(A)FE}}_{\text{“CTO”}}$ could be written as:
   - $a_4(\{\eta_i\}) = l_4 + 2e_7\bar{\eta} + e_8\eta_z$, $b_4(\{\eta_i\}) = m_4 + 2f_7\bar{\eta} + f_8\eta_z$;
   - $c_4(\{\eta_i\}) = n_4 + 2g_7\bar{\eta} + g_8\eta_z$, $c_5(\{\eta_i\}) = n_5 + 2g_9\bar{\eta} + g_{10}\eta_z$;
   - $c_6(\{\eta_i\}) = n_6 + 2g_{11}\bar{\eta} + g_{12}\eta_z$.

Then the energy for BFO-type structure is written as:

$$
\begin{aligned}
E_{\text{“BFO”}}(\{\eta_i\}) &= \underbrace{\alpha_1(\{\eta_i\})R^{\mathrm{O}^2} + \beta_1(\{\eta_i\})R^{\mathrm{O}^4} + \alpha_2(\{\eta_i\})\mathcal{T}^2 + \beta_2(\{\eta_i\})\mathcal{T}^4 + \gamma_1(\{\eta_i\})R^{\mathrm{O}^2}\mathcal{T}^2}_{E^{\mathrm{Rot}}_{\text{“BFO”}}} + \underbrace{\frac{1}{2}(2B_{11}\bar{\eta}^2 + B_{33}\eta_z^2) + 2B_{13}\bar{\eta}\eta_z + B_{12}\bar{\eta}^2}_{E^{\mathrm{Elas}}_{\text{“BFO”}}} \\
&\quad \underbrace{\begin{aligned}&+ \alpha_3(\{\eta_i\})\mathrm{FE_z}^2 + \beta_3(\{\eta_i\})\mathrm{FE_z}^4 + \alpha_4(\{\eta_i\})\mathrm{FE_{xy}}^2 + \beta_4(\{\eta_i\})\mathrm{FE_{xy}}^4 + \gamma_2(\{\eta_i\})\mathrm{FE_z}^2\mathrm{FE_{xy}}^2 + \gamma_3(\{\eta_i\})R^{\mathrm{O}^2}\mathrm{FE_z}^2 \\ &+ \gamma_4(\{\eta_i\})R^{\mathrm{O}^2}\mathrm{FE_{xy}}^2 + \gamma_5(\{\eta_i\})\mathcal{T}^2\mathrm{FE_z}^2 + \gamma_6(\{\eta_i\})\mathcal{T}^2\mathrm{FE_{xy}}^2 + \delta_1(\{\eta_i\})R^{\mathrm{O}}\mathcal{T}\mathrm{FE_z}\mathrm{FE_{xy}}\end{aligned}}_{E^{\mathrm{(A)FE}}_{\text{“BFO”}}} \\
&= E^{\mathrm{Rot}}_{\text{“BFO”}} + E^{\mathrm{Elas}}_{\text{“BFO”}} + E^{\mathrm{(A)FE}}_{\text{“BFO”}} \qquad \text{(S2)}
\end{aligned}
$$

Here we decompose the energy terms for BFO-type structure as follows:

1. The coefficients of these terms in $E^{\mathrm{Rot}}_{\text{“BFO”}}$ could be written as:
   - $\alpha_1(\{\eta_i\}) = \lambda_1 + 2\phi_1\bar{\eta} + \phi_2\eta_z$, $\alpha_2(\{\eta_i\}) = \lambda_2 + 2\phi_3\bar{\eta} + \phi_4\eta_z$;
   - $\beta_1(\{\eta_i\}) = \mu_1 + 2\chi_1\bar{\eta} + \chi_2\eta_z$, $\beta_2(\{\eta_i\}) = \mu_2 + 2\chi_3\bar{\eta} + \chi_4\eta_z$;

- $\gamma_1(\{\eta_i\}) = \nu_1 + 2\psi_1\bar{\eta} + \psi_2\eta_z$.

2. The coefficients of these terms in $E^{\text{(A)FE}}_{\text{“BFO”}}$ could be written as:

- $\alpha_3(\{\eta_i\}) = \lambda_3 + 2\phi_5\bar{\eta} + \phi_6\eta_z$, $\alpha_4(\{\eta_i\}) = \lambda_4 + 2\phi_7\bar{\eta} + \phi_8\eta_z$;
- $\beta_3(\{\eta_i\}) = \mu_3 + 2\chi_5\bar{\eta} + \chi_6\eta_z$, $\beta_4(\{\eta_i\}) = \mu_4 + 2\chi_7\bar{\eta} + \chi_8\eta_z$;
- $\gamma_2(\{\eta_i\}) = \nu_2 + 2\psi_3\bar{\eta} + \psi_4\eta_z$, $\gamma_3(\{\eta_i\}) = \nu_3 + 2\psi_5\bar{\eta} + \psi_6\eta_z$, $\gamma_4(\{\eta_i\}) = \nu_4 + 2\psi_7\bar{\eta} + \psi_8\eta_z$;
- $\gamma_5(\{\eta_i\}) = \nu_5 + 2\psi_9\bar{\eta} + \psi_{10}\eta_z$, $\gamma_6(\{\eta_i\}) = \nu_6 + 2\psi_{11}\bar{\eta} + \psi_{12}\eta_z$;
- $\delta_1(\{\eta_i\}) = \rho_1 + 2\omega_1\bar{\eta} + \omega_2\eta_z$.

The coefficients of expanded energy terms are determined from a series of first-principles total-energy calculations on distorted perovskite structures. For example, the coefficients $l_1$ and $m_1$ were obtained by introducing $R^{\mathrm{I}}$ distortion at nine different amplitudes into the cubic perovskite strutcures and fitting the energy to an even polynomial up to the fourth order. The two-body coupling parameters $n_1$ are determined by energy computations from 20 structures with two modes $R^{\mathrm{I}}$ and $\mathcal{T}$ varied in different amplitudes. When fitting $n_1$ the previous obtained coefficients $l_1$ and $m_1$ are kept unchanged. The coefficients of strain-dependent energy terms such as $e_1$ and $f_1$ relevant to $R^{\mathrm{I}}$ mode was extracted from a series of total-energy computations under nine incremental principal axial strains ranging from $-1\%$ to $1\%$. Energy fittings are performed with nine distorted structures for each applied strain. For other modes, their coefficients of self and two-body energy terms are obtained with similar technological processes for $R^{\mathrm{I}}$ and $\mathcal{T}$ modes. The coefficient of high-order energy term $o_1$ is fitted by energy computations for thirty structures with three modes $R^{\mathrm{I}}$, $\mathcal{T}$ and $\mathrm{AFE}_{xy}$ present. The coefficients of all self and two-body energy terms related to these three modes are kept the same values when fitting $o_1$. The coefficient $\rho_1$ for four-linear coupling energy terms can be determined with the similar approach. The coefficients about energy terms to describe how trilinear and fourlinear coupling interplays response to strain are also carried out under nine incremental principal axial strains ranging from $-1\%$ to $1\%$. Finally, elastic constants $B_{11}$, $B_{33}$, $B_{12}$ and $B_{13}$ are determined by a series of incremental principal axial strains applied on the cubic structure. The coefficients fitted for CTO-type and BFO-type structures of $CdHfO_3$ are listed in Table SI and Table SII respectively.

TABLE SI: The coefficients of Landau-type energy expansion for the CTO-type structure of $CdHfO_3$ fitted by first-principle calculations. The $l_1 \sim l_4$ and $e_1 \sim e_8$ are in unit of eV/Å$^2$; $m_1 \sim m_4$, $n_1 \sim n_6$, $f_1 \sim f_8$ and $g_1 \sim g_{12}$ are in unit of eV/Å$^4$; $o_1$, $h_1$ and $h_2$ are in unit of eV/Å$^3$. The unit of elasticity modulus is eV.

| $l_1$ | $m_1$ | $l_2$ | $m_2$ | $l_3$ | $m_3$ | $l_4$ | $m_4$ | $n_1$ | $n_2$ | $n_3$ | $n_4$ | $n_5$ | $n_6$ | $e_1$ | $e_2$ | $e_3$ |
|---|---|---|---|---|---|---|---|---|---|---|---|---|---|---|---|---|
| -2.943 | 1.253 | -2.839 | 0.814 | -1.013 | 0.893 | -1.021 | 0.222 | 0.727 | 0.492 | 0.524 | 0.486 | 0.453 | 0.075 | 10.422 | 7.169 | 8.776 |
| $e_4$ | $e_5$ | $e_6$ | $e_7$ | $e_8$ | $f_1$ | $f_2$ | $f_3$ | $f_4$ | $f_5$ | $f_6$ | $f_7$ | $f_8$ | $g_1$ | $g_2$ | $g_3$ | $g_4$ |
| 9.306 | -1.640 | 1.486 | 2.384 | -5.515 | -2.784 | 1.472 | -0.806 | -1.306 | -6.731 | -0.469 | -1.288 | -0.732 | -2.448 | -3.741 | -0.509 | -1.501 |
| $g_5$ | $g_6$ | $g_7$ | $g_8$ | $g_9$ | $g_{10}$ | $g_{11}$ | $g_{12}$ | $o_1$ | $h_1$ | $h_2$ | $B_{11}$ | $B_{12}$ | $B_{13}$ | $B_{33}$ | | |
| -0.290 | -1.898 | -3.240 | -4.281 | -1.948 | -0.559 | 0.589 | 5.674 | -0.426 | 3.750 | 3.557 | 572.16 | 183.28 | 189.15 | 582.81 | | |

TABLE SII: The coefficients of Landau-type energy expansion for the BFO-type structure of $CdHfO_3$ fitted by first-principle calculations. The $\lambda_1 \sim \lambda_4$ and $\phi_1 \sim \phi_8$ are in unit of eV/Å$^2$; $\mu_1 \sim \mu_4$, $\nu_1 \sim \nu_6$, $\chi_1 \sim \chi_8$ and $\psi_1 \sim \psi_{12}$ are in unit of eV/Å$^4$; $\rho_1$, $\omega_1$ and $\omega_2$ are in unit of eV/Å$^4$. The unit of elasticity modulus is eV.

| $\lambda_1$ | $\mu_1$ | $\lambda_2$ | $\mu_2$ | $\lambda_3$ | $\mu_3$ | $\lambda_4$ | $\mu_4$ | $\nu_1$ | $\nu_2$ | $\nu_3$ | $\nu_4$ | $\nu_5$ | $\nu_6$ | $\phi_1$ | $\phi_2$ | $\phi_3$ |
|---|---|---|---|---|---|---|---|---|---|---|---|---|---|---|---|---|
| -2.911 | 1.276 | -2.839 | 0.814 | -1.021 | 0.222 | -1.311 | 0.348 | 0.795 | 0.521 | 0.499 | 0.655 | 0.453 | 0.426 | 10.239 | 7.039 | 8.776 |
| $\phi_4$ | $\phi_5$ | $\phi_6$ | $\phi_7$ | $\phi_8$ | $\chi_1$ | $\chi_2$ | $\chi_3$ | $\chi_4$ | $\chi_5$ | $\chi_6$ | $\chi_7$ | $\chi_8$ | $\psi_1$ | $\psi_2$ | $\psi_3$ | $\psi_4$ |
| 9.306 | 2.384 | -5.515 | -2.251 | 1.664 | -2.625 | 2.741 | -0.806 | -1.306 | -1.288 | -0.732 | -1.844 | -0.542 | -2.345 | -2.831 | -2.533 | -5.294 |
| $\psi_5$ | $\psi_6$ | $\psi_7$ | $\psi_8$ | $\psi_9$ | $\psi_{10}$ | $\psi_{11}$ | $\psi_{12}$ | $\rho_1$ | $\omega_1$ | $\omega_2$ | $\mathrm{B}_{11}$ | $\mathrm{B}_{12}$ | $\mathrm{B}_{13}$ | $\mathrm{B}_{33}$ | | |
| -3.215 | -4.270 | -1.048 | -2.855 | -1.948 | -0.559 | -0.429 | -2.910 | -0.722 | 5.454 | 11.823 | 572.16 | 183.28 | 189.15 | 582.81 | | |

## III. MODEL RELIABILITY ANALYSIS

In the main text, we have made a comparison for DFT and model calculated relative energy between CTO-type and BFO-type structures of $CdHfO_3$ as a function of epitaxial strain, which demonstrates the capability of model to describe the structural transition from energy aspect. In order to future verify the reliability of our constructed model,

we plotted amplitudes of phonon modes frozen in CTO-type and BFO-type structures varied with epitaxial strain. As shown in Fig. S1(a), DFT calculated amplitudes of octahedral rotations in CTO-type and BFO-type structures are quite similar and varied slightly with strain, hardly contributing to the stabilization of BFO-type structure. However, the amplitude of antipolar mode in CTO-type structure decreases rapidly with strain but ferroelectric mode in BFO-type structure shows a significantly increased amplitude with strain, which play a decisive role to attain BFO-type structure. The modeling results in Fig. S1(b) mostly conform to those of DFT, indicating our constructed model can capture the origin of the transition between CTO-type and BFO-type structures as well. The main energy error in Fig. 1(a) of main text arises from the amplitude of antipolar mode under large strain, showing a evident difference between DFT and modeling results. This problem may be solved by including more high order energy terms, but it does not affect the key physical picture in current work.

## IV. ENERGY CALCULATED BY PAW AND NC PSEUDOPOTENTIAL

In this work, the DFT simulations without electric boundary condition and model Hamiltonian fittings are performed with the projector augmented wave (PAW) pseudopotential, whereas the electric displacement field calculations are carried out with the norm-conservation (NC) pseudopotential. Since PAW and NC pseudopotentials possess the different transferability to various chemical environments and different energy cutoff for kinetic energy truncation, it is necessary to compare relative energy between CTO-type and BFO-type structures calculated from different pseudopotentials. The NC pseudopotentials are constructed based on the Vanderbilt introduced ultrasoft pseudopotential approach without forfeiting the norm conservation. This type of NC pseudopotentials with a multiple-projector prescription could reproduce scattering properties to all-electron results more accurately and just moderately increased plane-wave energy cutoff. As shown in the Table SIII, the relative energies between CTO-type and BFO-type structures for five perovsktites are quite similar for NC and PAW pseudopotential calculations, which is crucial to determine the stabilization of BFO-type structure.

TABLE SIII: The relative energy(in meV) between CTO-type and BFO-type structures for five perovsktites calculated with NC and PAW pseudopotentials.

| | $CdHfO_3$ | $CdSnO_3$ | $NaMnF_3$ | $CaZrO_3$ | $CaHfO_3$ |
|---|---|---|---|---|---|
| NC | 49 | 141 | 85 | 214 | 280 |
| PAW | 41 | 123 | 74 | 202 | 297 |

## V. STRUCTURE SEARCH BASED ON GENETIC ALGORITHM

Genetic algorithm is an optimization strategy similar to the Darwinian evolution process that employs natural selection of the fittest child structures through the mating and mutation operations on parent structures. Starting with a population of candidate structures as the first generation, then optimizing these candidates to the nearest local minimum. Among the locally optimized structures, a certain number of the worst ones are abandoned, and the rest of structures participate in creating the next generation through selection operations. This process is repeated until the ground state structure is searched. Since all distorted perovskite structures are evoluted from the undistorted cubic structure, the first generation are created by random selection of initial structures belonging to the subgroup of the cubic structure in our work. The cut and splice crossover operator proposed by Deaven and Ho are considered as the mating operation, which is expressed as:

$$X_{\mathrm{child}} = X_{\mathrm{cubic}} + (X_{\mathrm{father}} - X_{\mathrm{cubic}}) + c(X_{\mathrm{mother}} - X_{\mathrm{cubic}}).$$

where $X_{\mathrm{father}}$ and $X_{\mathrm{mother}}$ are the two parent structures, $X_{\mathrm{cubic}}$ and $X_{\mathrm{child}}$ represent the undistorted cubic structure and new child structure. The constant $c$ is randomly chosen to be 1 or -1. The parent structures with lower energy are preferentially to be selected. The probability to be selected for mating is given by the Boltzmann distribution. The first four searched low-energy structures for CTO-type perovekites are listed in Tables SIV. Table SV shows the searched low-energy structures for $EuZrO_3$ and $EuHfO_3$ undr tensile 5% strain.

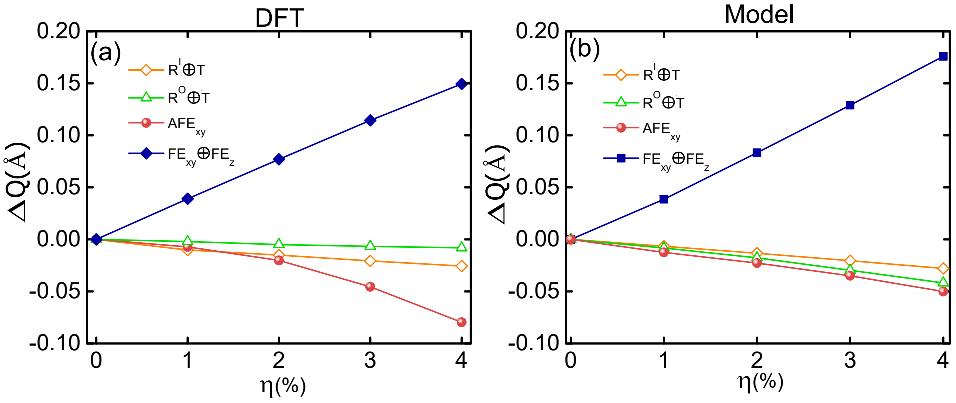


FIG. S1: (color online) The amplitudes of phonon modes as a function of applied epitaxial strain. (a) and (b) describe the results obtained from DFT calculations and effective Hamiltonian modes respectively. $R^{\mathrm{I}} \bigoplus \mathcal{T}$ and $R^{\mathrm{O}} \bigoplus \mathcal{T}$ denote octahedral rotations in CTO-type and BFO-type structures; $\mathrm{AFE}_{xy}$ stands for the antipolar mode in CTO-type structure; and $\mathrm{FE}_{xy} \bigoplus \mathrm{FE}_z$ represent both in-plane and out-of-plane ferroelectric modes in BFO-type structure. The amplitudes of all phonon modes are set to zero at strain-free states.

TABLE SIV: DFT calculated total energies of the ground state and first four metastable structures for perovskite materials studied in this work. The energy is given out relative to that of ground state and in unit of meV. Space group symbols are also shown for all structures. Structures with $\mathrm{P2_1/c^{(1)}}$ and $\mathrm{P2_1/c^{(2)}}$ symmetries mean their space configurations are different but belongs to the same space group.

| order / Mat. | Ground state | | $1^{st}$-metastable | | $2^{nd}$-metastable | | $3^{rd}$-metastable | | $4^{th}$-metastable | |
|---|---|---|---|---|---|---|---|---|---|---|
| | Sym. | $\Delta E$(meV) | Sym. | $\Delta E$(meV) | Sym. | $\Delta E$(meV) | Sym. | $\Delta E$(meV) | Sym. | $\Delta E$(meV) |
| $CdHfO_3$ | Pnma | 0 | R3c | 41 | $P2_1/c^{(1)}$ | 157 | C2/c | 223 | $R\bar{3}c$ | 227 |
| $CdSnO_3$ | Pnma | 0 | R3c | 123 | $P2_1/c^{(1)}$ | 327 | $P2_1/c^{(2)}$ | 335 | $R\bar{3}c$ | 346 |
| $CdTiO_3$ | $Pna2_1$ | 0 | R3c | 95 | $P2_1/c^{(1)}$ | 259 | $R\bar{3}c$ | 261 | Imma | 269 |
| $CaZrO_3$ | Pcmn | 0 | R3c | 202 | $P2_1/c^{(1)}$ | 491 | Imma | 511 | $P2_1/c^{(2)}$ | 649 |
| $CaHfO_3$ | Pnma | 0 | R3c | 297 | Imma | 457 | $P2_1/c^{(1)}$ | 507 | $P2_1/c^{(2)}$ | 513 |
| $ScCrO_3$ | Pnma | 0 | R3c | 44 | $P2_1/c^{(1)}$ | 1529 | Imma | 1751 | C2/c | 2260 |
| $EuZrO_3$ | Pbnm | 0 | Imma | 121 | $P2_1/c^{(1)}$ | 183 | R3c | 188 | $P2_1/c^{(2)}$ | 195 |
| $EuHfO_3$ | Pbnm | 0 | Imma | 71 | $P2_1/c^{(1)}$ | 110 | $P2_1/c^{(2)}$ | 116 | R3c | 120 |
| $LuFeO_3$ | Pbnm | 0 | R3c | 820 | $P2_1/c^{(1)}$ | 1399 | Imma | 1537 | $P2_1/c^{(2)}$ | 1762 |
| $NaMnF_3$ | Pnma | 0 | R3c | 74 | $P2_1/c^{(1)}$ | 216 | Imma | 242 | $P2_1/c^{(2)}$ | 264 |

TABLE SV: DFT calculated total energies and space group symbols of the ground state and first four metastable structures for 5% strained $EuZrO_3$ and $EuHfO_3$ perovskites. The energy is given out relative to that of ground state and in unit of meV.

| order / Mat. | Ground state | | $1^{st}$-metastable | | $2^{nd}$-metastable | | $3^{rd}$-metastable | | $4^{th}$-metastable | |
|---|---|---|---|---|---|---|---|---|---|---|
| | Sym. | $\Delta E$(meV) | Sym. | $\Delta E$(meV) | Sym. | $\Delta E$(meV) | Sym. | $\Delta E$(meV) | Sym. | $\Delta E$(meV) |
| $EuZrO_3$ | R3c | 0 | Pbnm | 101 | $P2_1/c^{(1)}$ | 137 | $R\bar{3}c$ | 138 | Cmcm | 272 |
| $EuHfO_3$ | R3c | 0 | Pbnm | 39 | $P2_1/c^{(1)}$ | 51 | $R\bar{3}c$ | 52 | Cmcm | 129 |

## VI. STABILIZE BFO-TYPE STRUCTURE IN GENERAL PEROVSKITE MATERIALS

In this section, we generalize the design mechanism learned from $CdHfO_3$ to the widely spread perovskite materials which naturally exist as CTO-type structure. It can be inferred that there are two prerequisites before a CTO-type perovskite can be engineered into BFO-type structure with functional FE polarizations. Firstly, this perovskite possesses a hidden polar instability in addition to the oxygen octahedral rotation and tilt. The above can be confirmed by the predicted phonon dispersion for the perovskite at the hypothetical high-temperature phase with cubic symmetry from first-principles. The frequencies of major unstable phonons for cubic $\mathrm{Pm\bar{3}m}$ structures of perovskite materials studied in this work are listed in Table SVI. In the case of cubic $CdHfO_3$ of $Pm\bar{3}m$ space group symmetry, the three lowest unstable phonon modes are identified to at the $\Gamma(\omega = 149i)$, $M(\omega = 337i)$, and $R(\omega = 327i)$, points of the Brillouin Zone, which give rise to the polar, in-phase oxygen octahedral rotation, and oxygen octahedral tilt

distortion, respectively. At ground state $CdHfO_3$ adopts the CTO-type structure with an improper AFE distortion via the trilinear coupling mechanism. Due to the above hidden polar instability, FE ordering becomes a competing structure which can be stabilized by the improper four-linear coupling mechanism under adjustable mechanical and electric boundary conditions as described in the above. Secondly, the BFO-type structure should be the metastable state as the second lowest DFT energy as shown in Table SIV. Moreover, the energy barrier between BFO-type structure and its ground state CTO-type structure should be small. As far as $CdHfO_3$ is concerned, the total DFT energy difference between the CTO-type and BFO-type structures is about 10 meV/formula, which indeed facilities the stabilization of its metastable phase as described above.

With the above two guidelines, we have done a survey on the databased of perovskites with CTO-type as ground state structure [S13]. In the above, we have identified nine perovskites that have intrinsic polar instabilities in their cubic phases. We then further employ the genetic evolutionary algorithm [S14] to determine their potential metastable structures as well as their energetics. Seven of nine perovskites are found to have BFO-type structure as the lowest-energy metastable phase. As shown in in Table SVII, we present the seven candidates of perovskite that satisfy the above criteria. At ground state, these materials have space group symmetries of $Pnma$ ($CdHfO_3$, $CdSnO_3$, $CaHfO_3$, $SrCrO_3$, and $NaMnF_3$), $Pna2_1$($CdTiO_3$), $Pcmn$ ($CaZrO_3$), and $Pbnm$ ($LuFeO_3$) respectively. In their structure, the distortions include a typical in-phase octahedral rotation around the long crystal axis (assumed to be the out-of-plane of $c$ direction) and octahedral tilt around the in-plane direction composed by the two short axes ($a$ and $b$). Therefore, in-plane antipolar distortions develop in all these seven perovskites due to the improper trilinear coupling mechanism. All the seven candidates are non-polar at ground state except for the $CdTiO_3$ [S15], which develop a polarization along out-of-plane direction allowed by its space group symmetry ($Pna2_1$). Nevertheless, based on their structural distortions, all these perovskites can be characterized as CTO-type structures in their natural bulks.

TABLE SVI: Calculated lowest phonon frequencies ($cm^{-1}$) for the cubic perovskite materials at the $\Gamma$, $X$, $M$, and $R$ points of the Brillouin Zone.

| mode \ Mat. | $CdHfO_3$ | $CdSnO_3$ | $CdTiO_3$ | $CaZrO_3$ | $CaHfO_3$ | $SrCrO_3$ | $EuZrO_3$ | $EuHfO_3$ | $LuFeO_3$ | $NaMnF_3$ |
|---|---|---|---|---|---|---|---|---|---|---|
| $\Gamma_4^-$ | 149i | 142i | 144i | 177i | 162i | 272i | 92i | 60i | 196i | 97i |
| $X_5^+$ | 103i | 133i | 40i | 120i | 108i | 262i | 17i | 28i | 126i | 71i |
| $M_3^+$ | 337i | 353i | 308i | 233i | 228i | 354i | 176i | 162i | 324i | 140i |
| $R_5^-$ | 327i | 352i | 303i | 239i | 234i | 379i | 193i | 183i | 350i | 141i |

TABLE SVII: Computed electric polarizations ($\mu C/cm^2$) in the in-plane ($P_\parallel$) and out-of-plane directions($P_\perp$). $\Delta E$ is the computed energy difference in unit of meV between the CTO-type structure at ground state and the metastable BFO-type structure. $\eta_c$ denotes the critical tensile epitaxial to stabilize the perovskite into BFO-type structure.

| Mat. | Bulk | | | | | | Strained Bulk | | | | |
|---|---|---|---|---|---|---|---|---|---|---|---|
| | CTO-type | | | BFO-type | | | CTO-type | | BFO-type | | |
| | Ground state | | | Metastable | | | Metastable | | Ground state | | |
| | Sym. | $P_\parallel$ ($\mu C/cm^2$) | $P_\perp$ ($\mu C/cm^2$) | $P_\parallel$ ($\mu C/cm^2$) | $P_\perp$ ($\mu C/cm^2$) | $\Delta E$(meV) | $P_\parallel$ ($\mu C/cm^2$) | $P_\perp$ ($\mu C/cm^2$) | $P_\parallel$ ($\mu C/cm^2$) | $P_\perp$ ($\mu C/cm^2$) | $\eta_c$(%) |
| $CdHfO_3$ [S16] | Pnma | 0 | 0 | 34.1 | 24.1 | 41 | 0 | 0 | 30.2 | 20.4 | 2.3 |
| $CdSnO_3$ [S17] | Pnma | 0 | 0 | 32.0 | 22.6 | 123 | 0 | 11.4 | 28.6 | 21.7 | 2.4 |
| $CdTiO_3$ [S15] | $Pna2_1$ | 0 | 20.82 | 50.5 | 35.7 | 95 | 46.78 | 0 | 61.7 | 25.0 | 2.8 |
| $CaZrO_3$ [S18] | Pcmn | 0 | 0 | 41.2 | 28.5 | 202 | 0 | 0 | 36.8 | 24.6 | 3.0 |
| $CaHfO_3$ [S19] | Pnma | 0 | 0 | 35.0 | 24.5 | 297 | 0 | 0 | 40.4 | 20.8 | 3.5 |
| $ScCrO_3$ [S20] | Pnma | 0 | 0 | 64.3 | 44.5 | 44 | 0 | 0 | 60.4 | 43.8 | 2.4 |
| $LuFeO_3$ [S21] | Pbnm | 0 | 0 | 65.2 | 45.2 | 820 | 0 | 0 | 70.4 | 42.4 | 5.1 |
| $NaMnF_3$ [S7] | Pnma | 0 | 0 | 19.3 | 13.5 | 74 | 0 | 5.7 | 18.4 | 12.1 | 3.0 |

We first apply the adjustable mechanical boundary condition to stabilize the BFO-type structure by using the epitaxial tensile strain on the perovskites. To this end, we perform direct DFT calculations by gradually increasing the magnitudes of tensile strains applied on the perovskite until the critical strain $\eta_c$ is reached as $\Delta F(\eta) > 0$. It indicates the BFO-type structure becomes more stable than the CTO-type structure. The resulting electric polarizations as well as the critical strains $\eta_c$ are presented in Table SVII. Clearly, it can be seen that all the seven perovskites can be

stabilized into BFO-type structures if the applied tensile strain is large enough. In BFO-type structure, distortions are characterized by a large out-of-phase octahedral rotation. Because of the four-linear coupling, the improper FE mode develops along both out-of-plane and in-plane direction as shown in Table SVII. In the same table, we also present the Kohn-Sham energy difference $\Delta E$ between the CTO-type structure of ground state and the BFO-type structure as the metastable state computed by DFT. It can be noted that $\eta_c$ is inversely proportional to the $\Delta E$ in the perovskite in the absence of spin-order as shown in Table SVII. On the other hand, the $\Delta E$ in the perovskite in the multiferroic perovskite can be further affected by the spin-phonon coupling effect.

We then proceed to apply the approach by using proper electric boundary conditions to stabilize the BFO-type structure. In particular, we carry out constrained $\boldsymbol{D}$-field DFT calculations by using the two perovskites of $CdSnO_3$ and $NaMnF_3$ in Table SIV as the examples to demonstrate the mechanism. The changes of free energy $\Delta F(\boldsymbol{D})$ as a function of electric displacement field are presented in Figs. S2(a) and S2(b) for $CdSnO_3$ and $NaMnF_3$, respectively. Qualitatively to the case of $CdHfO_3$ in Fig. 1(b), both $CdSnO_3$ and $NaMnF_3$ can be stabilized to be BFO-type structure with applied electric displacement field $\boldsymbol{D}$ = 0.25C/m$^2$ and $\boldsymbol{D}$ = 0.17C/m$^2$ respectively. It can be noted that $CdSnO_3$ requires a larger electric displacement field to stabilize its metastable phase than $NaMnF_3$ does. The above fact is also consistent with the higher energy barrier of $CdSnO_3$ than that of $NaMnF_3$ as reported in Table SVII.

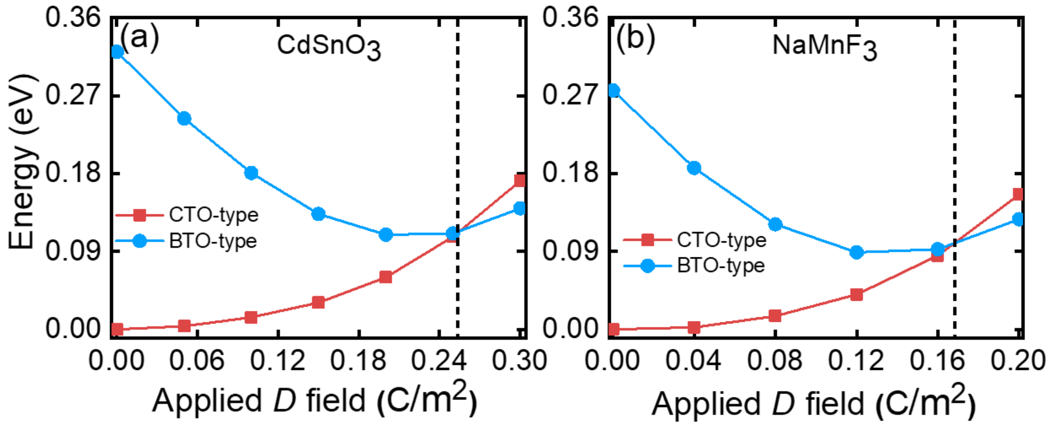


FIG. S2: The energies of DFT under constrained electric displacement field ($\boldsymbol{D}$) in (a)$CdSnO_3$, (b) $NaMnF_3$. The energy of CTO-type structure under zero $\boldsymbol{D}$ field is set to the reference energy in each plot.

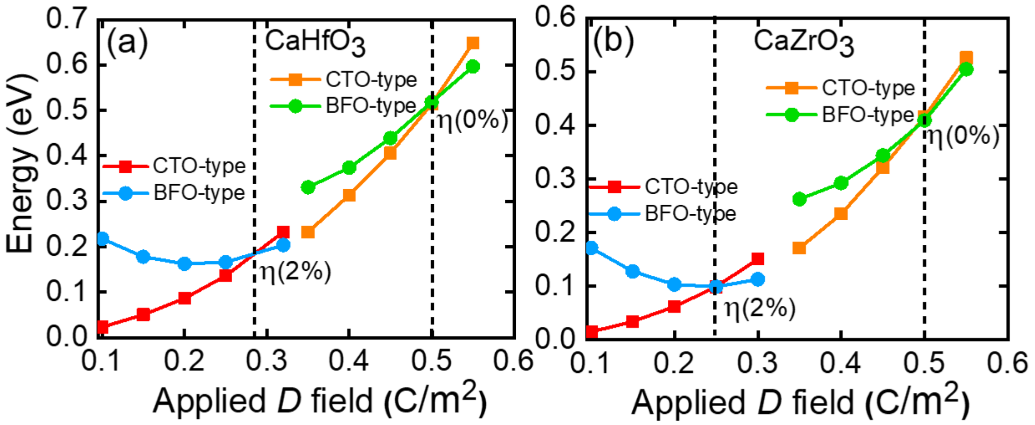


FIG. S3: DFT calculated internal energy as a function of $\boldsymbol{D}$ field for (a)$CaHfO_3$ and (b)$CaZrO_3$. The constrained $\boldsymbol{D}$ field simulations for $CaHfO_3$ and $CaZrO_3$ are performed without strain and with 2% tensile strain respectively. The energy of CTO-type structure under zero $\boldsymbol{D}$ field is set to the reference energy in each plot.

By combining the mechanical and electric boundary conditions, the critical strain and $\boldsymbol{D}$-field required to stabilize the BFO-type structure can be both further optimized. Our first-principles calculations show that as large as $\boldsymbol{D}$ = 0.50C/m$^2$ and $\boldsymbol{D}$ = 0.50C/m$^2$ are required to stabilize BFO-type structure in $CaHfO_3$ and $CaZrO_3$ by using applied

electric displacement field only. See Figure S3. However, with combined mechanical and electric boundary conditions, the critical $\boldsymbol{D}$-fields are largely reduced to $\boldsymbol{D}$ = 0.28C/m$^2$ and $\boldsymbol{D}$ = 0.25C/m$^2$ respectively for $CaHfO_3$ and $CaZrO_3$ under 2% epitaxial stain. In experiments, it should be noted that the applied $\boldsymbol{D}$-field can be realized either by externally applied electric fields; or achieved by growing highly polar component in perovskite superlattice via the electrostatic coupling effect.

---


[S1] R. O. Jones, Rev. Mod. Phys. **87**, 897 (2015).
[S2] G. Kresse and J. Hafner, Phys. Rev. B **47**, 558 (1993).
[S3] G. Kresse and D. Joubert, Phys. Rev. B **59**, 1758 (1999).
[S4] J. P. Perdew, A. Ruzsinszky, G. I. Csonka, O. A. Vydrov, G. E. Scuseria, L. A. Constantin, X. Zhou, and K. Burke, Phys. Rev. Lett. **100**, 136406 (2008).
[S5] P. E. Blöchl, Phys. Rev. B **50**, 17953 (1994).
[S6] J. Hong, A. Stroppa, J. Íniguez, S. Picozzi, and D. Vanderbilt, Phys. Rev. B **85**, 054417 (2012).
[S7] A. C. Garcia-Castro, A. H. Romero, and E. Bousquet, Phys. Rev. Lett. **116**, 117202 (2016).
[S8] A. Togo and I. Tanaka, Scr. Mater. **108**, 1 (2015).
[S9] D. Xiao, M.-C. Chang, and Q. Niu, Rev. Mod. Phys. **82**, 1959 (2010).
[S10] X. Gonze, B. Amadon, P.-M. Anglade, J.-M. Beuken, F. Bottin, P. Boulanger, F. Bruneval, D. Caliste, R. Caracas, M. Côté, et al., Comput. Phys. Commun **180**, 2582 (2009).
[S11] D. Hamann, Phys. Rev. B **88**, 085117 (2013).
[S12] X. Lu, X. Gong, and H. Xiang, Computational Materials Science **91**, 310 (2014), ISSN 0927-0256.
[S13] A. Jain, S. P. Ong, G. Hautier, W. Chen, W. D. Richards, S. Dacek, S. Cholia, D. Gunter, D. Skinner, G. Ceder, et al., APL materials **1**, 011002 (2013).
[S14] H. J. Xiang, S.-H. Wei, and X. G. Gong, Phys. Rev. B **82**, 035416 (2010).
[S15] H. Moriwake, A. Kuwabara, C. A. J. Fisher, H. Taniguchi, M. Itoh, and I. Tanaka, Phys. Rev. B **84**, 104114 (2011).
[S16] N. Shpilevaya, M. Kupriyanov, B. Kul'buzhev, and Y. V. Kabirov, Phys. Solid State **46**, 2263 (2004).
[S17] H. Mizoguchi, H. W. Eng, and P. M. Woodward, Inorg. Chem. **43**, 1667 (2004).
[S18] P. Stoch, J. Szczerba, J. Lis, D. Madej, and Z. Pedzich, J. Eur. Ceram. Soc. **32**, 665 (2012).
[S19] A. Feteira, D. C. Sinclair, K. Z. Rajab, and M. T. Lanagan, J. Am. Ceram. Soc. **91**, 893 (2008).
[S20] A. A. Belik, Y. Matsushita, M. Tanaka, and E. Takayama-Muromachi, Chem. Mater. **24**, 2197 (2012).
[S21] U. Chowdhury, S. Goswami, D. Bhattacharya, J. Ghosh, S. Basu, and S. Neogi, Appl. Phys. Lett **105**, 052911 (2014).
